# Supplementary material for: On-Device Training Under 256KB Memory
Source: arXiv:2206.15472 source file (2024-04-03)
Supplement: Supplementary file 1 [file supp.tex]

\documentclass{article}

\input{package}
\usepackage{minted}
\input{macro}

\title{
Supplementary Material\\ On-Device Training Under 256KB Memory }

\begin{document}

\maketitle
{
  \hypersetup{linkcolor=black}
  \tableofcontents
}
\renewcommand{\thefigure}{S\arabic{figure}}
\renewcommand{\thetable}{S\arabic{table}}
\newpage

\appendix
\input{text/appendix}

\newpage
\small
\bibliographystyle{plain}
\bibliography{main}

\end{document}
